# Supplementary material for: Beyond ELBOs: A Large-Scale Evaluation of Variational Methods for Sampling
Source: arXiv:2406.07423 source file (2024-06-11)
Supplement: Supplementary file 1 [file network.tex]

\subsection{Ablation Study: Network Architecture} \label{abl:network}
%%%%%%%%%%%%%%%%%%%%%%%%%%%%%%%%%%%%%%%%%%%%%%%%%%%%%%%%%%%%%%%%%%%%%%%%%%%%%%%%%
\textbf{Experimental Setup.} We compare the network architecture proposed by 
\cite{geffner2022langevin} and \cite{zhang2021path} with different number of hidden layer for MCD \cite{doucet2022annealed} on the MoG target. The main difference between these architectures is that \cite{zhang2021path} use a sinusoidal position embedding for the time while \cite{geffner2022langevin} uses random features for embedding the time. Results are shown in Table \ref{abl_network} 

\textbf{Discussion.} 
% The results comparing \cite{geffner2022langevin} Score Network with \cite{zhang2021path} PIS Network are presented in Table \ref{abl_network} regarding \red{Todo}. 
Surprisingly increasing the number of layer of the networks tends to lead to worse performance in high dimensions. Moreover, the results are mixed as to which time embedding is preferable.
%%%%%%%%%%%%%%%%%%%%%%%%%%%%%%%%%%%%%%%%%%%%%%%%%%%%%%%%%%%%%%%%%%%%%%%%%%%%%%%%%
\begin{table*}[h!]
% \caption{\textbf{VI Results.} $ \log Z$ values for a different number of steps $K$.}
\begin{center}
\begin{small}
\begin{sc} {
\resizebox{\textwidth}{!}{%
\begin{tabular}{c|c|ccc|ccc}
\toprule
  \textbf{Network} & & \multicolumn{3}{c|}{\textbf{ELBO} $\uparrow$} & \multicolumn{3}{c}{\textbf{EMC} $\uparrow$}   \\ 
\textbf{Architecture} & \textbf{Layers}  & $d=2$ & $d=50$  & $d=200$ & $d=2$ & $d=50$  & $d=200$   \\ 
\midrule
% \multicolumn{10}{c}{\underline{ELBO}} \\
%%%%%%%%%%%%%%%%%%%%%%%%%%%%%%%%%%%%%%%%%%%%%%%%%%%%%%%%%%%%%%%%%%%%%%%%%%%%%%%%%%%%%%%%
\cite{geffner2022langevin}
& 2
& $-2.384 \scriptstyle \pm 0.059$ % ELBO d=2
& $-878.12 \scriptstyle \pm 8.598$ % ELBO d=50
& $\mathbf{-3610.809 \scriptstyle \pm 278.257}$ % ELBO d=200
& $0.798 \scriptstyle \pm 0.003$ % EUBO d=2
& $0.994 \scriptstyle \pm 0.001$ % EUBO d=50
& $0.988 \scriptstyle \pm 0.0$ % EUBO d=200
\\
%%%%%%%%%%%%%%%%%%%%%%%%%%%%%%%%%%%%%%%%%%%%%%%%%%%%%%%%%%%%%%%%%%%%%%%%%%%%%%%%%%%%%%%%
& 4
& $-1.875 \scriptstyle \pm 0.057$ % ELBO d=2
& $\mathbf{-823.108 \scriptstyle \pm 21.124}$ % ELBO d=50
& $-4269.703 \scriptstyle \pm 383.171$ % ELBO d=200
& $0.8 \scriptstyle \pm 0.002$ % EUBO d=2
& $0.994 \scriptstyle \pm 0.001$ % EUBO d=50
& $0.988 \scriptstyle \pm 0.001$ % EUBO d=200
\\
%%%%%%%%%%%%%%%%%%%%%%%%%%%%%%%%%%%%%%%%%%%%%%%%%%%%%%%%%%%%%%%%%%%%%%%%%%%%%%%%%%%%%%%%
& 6
& $\mathbf{-1.856 \scriptstyle \pm 0.145}$ % ELBO d=2
& $-832.888 \scriptstyle \pm 12.31$ % ELBO d=50
& $-5655.213 \scriptstyle \pm 502.352$ % ELBO d=200
& $0.8 \scriptstyle \pm 0.002$ % EUBO d=2
& $0.994 \scriptstyle \pm 0.0$ % EUBO d=50
& $0.989 \scriptstyle \pm 0.0$ % EUBO d=200
\\
\midrule
% %%%%%%%%%%%%%%%%%%%%%%%%%%%%%%%%%%%%%%%%%%%%%%%%%%%%%%%%%%%%%%%%%%%%%%%%%%%%%%%%%%%%%%%%
\cite{zhang2021path}
& 2
& $-1.545 \scriptstyle \pm 0.039$ % ELBO d=2
& $\mathbf{-1161.208 \scriptstyle \pm 101.582}$ % ELBO d=50
& $\mathbf{-37063.991 \scriptstyle \pm 90.883}$ % ELBO d=200
& $0.801 \scriptstyle \pm 0.001$ % EUBO d=2
& $0.994 \scriptstyle \pm 0.001$ % EUBO d=50
& $0.988 \scriptstyle \pm 0.001$ % EUBO d=200
\\
%%%%%%%%%%%%%%%%%%%%%%%%%%%%%%%%%%%%%%%%%%%%%%%%%%%%%%%%%%%%%%%%%%%%%%%%%%%%%%%%%%%%%%%%
& 4
& $-1.219 \scriptstyle \pm 0.061$ % ELBO d=2
& $-1281.489 \scriptstyle \pm 104.318$ % ELBO d=50
& $-38194.788 \scriptstyle \pm 166.082$ % ELBO d=200
& $0.801 \scriptstyle \pm 0.002$ % EUBO d=2
& $0.994 \scriptstyle \pm 0.0$ % EUBO d=50
& $0.989 \scriptstyle \pm 0.001$ % EUBO d=200
\\
%%%%%%%%%%%%%%%%%%%%%%%%%%%%%%%%%%%%%%%%%%%%%%%%%%%%%%%%%%%%%%%%%%%%%%%%%%%%%%%%%%%%%%%%
& 6
& $\mathbf{-1.139 \scriptstyle \pm 0.023}$ % ELBO d=2
& $-1200.573 \scriptstyle \pm 179.776$ % ELBO d=50
& $-40336.673 \scriptstyle \pm 153.416$ % ELBO d=200
& $0.801 \scriptstyle \pm 0.002$ % EUBO d=2
& $0.994 \scriptstyle \pm 0.0$ % EUBO d=50
& $0.988 \scriptstyle \pm 0.001$ % EUBO d=200
\\
% %%%%%%%%%%%%%%%%%%%%%%%%%%%%%%%%%%%%%%%%%%%%%%%%%%%%%%%%%%%%%%%%%%%%%%%%%%%%%%%%%%%%%%%%
\bottomrule
\end{tabular}
}}
\end{sc}
\end{small}
\end{center}
\vskip -0.1in
\caption{ELBO and EMC values for network architectures proposed by \cite{geffner2022langevin} and \cite{zhang2021path} with different number of hidden layer for MCD \cite{doucet2022annealed} on the MoG target. The main difference between these architectures is that \cite{zhang2021path} use a sinusoidal position embedding for the time while \cite{geffner2022langevin} use random features.}
\label{abl_network}
\end{table*}
%%%%%%%%%%%%%%%%%%%%%%%%%%%%%%%%%%%%%%%%%%%%%%%%%%%%%%%%%%%%%%%%%%%%%%%%%%%%%
