# Supplementary material for: Beyond ELBOs: A Large-Scale Evaluation of Variational Methods for Sampling
Source: arXiv:2406.07423 source file (2024-06-11)
Supplement: Supplementary file 2 [file loss_fn.tex]

\subsection{Ablation Study: Loss-Function} \label{abl:loss_fn}
%%%%%%%%%%%%%%%%%%%%%%%%%%%%%%%%%%%%%%%%%%%%%%%%%%%%%%%%%%%%%%%%%%%%%%%%%%%%%%%%%
\textbf{Experimental Setup.} \cite{richter2023improved} proposed to use VarGrad \cite{richter2020vargrad} as an alternative to maximizing the ELBO. They showed that VarGrad helps with mode collapse. Here, we compare ELBO and Vargrad on the MoG target for DDS and CMCD for a varying number of dimensions. The results are shown in Table \ref{abl_loss}.

\textbf{Discussion.} We generally observe higher EMC values using VarGrad. However, they come with the cost of significantly higher looseness in the ELBO.

%%%%%%%%%%%%%%%%%%%%%%%%%%%%%%%%%%%%%%%%%%%%%%%%%%%%%%%%%%%%%%%%%%%%%%%%%%%%%%%%%
\begin{table*}[h!]
% \caption{\textbf{VI Results.} $ \log Z$ values for a different number of steps $K$.}
\begin{center}
\begin{small}
\begin{sc} {
\resizebox{\textwidth}{!}{%
\begin{tabular}{l|c|ccc|ccc}
\toprule
   &   & \multicolumn{3}{c|}{\textbf{ELBO} $\uparrow$} & \multicolumn{3}{c}{\textbf{EMC} $\uparrow$}   \\ 
 \textbf{Method} & \textbf{Loss}  & $d=2$ & $d=50$  & $d=200$ & $d=2$ & $d=50$  & $d=200$   \\ 
\midrule
% \multicolumn{10}{c}{\underline{ELBO}} \\
%%%%%%%%%%%%%%%%%%%%%%%%%%%%%%%%%%%%%%%%%%%%%%%%%%%%%%%%%%%%%%%%%%%%%%%%%%%%%%%%%%%%%%%%
DDS
& ELBO
& $\mathbf{-0.612 \scriptstyle \pm 0.019}$ % ELBO d=2
& $\mathbf{-15.598 \scriptstyle \pm 0.106}$ % ELBO d=50
& $\mathbf{-63.101 \scriptstyle \pm 0.253}$ % ELBO d=200
& $\mathbf{0.984 \scriptstyle \pm 0.001}$ % EUBO d=2
& $\mathbf{0.992 \scriptstyle \pm 0.001}$ % EUBO d=50
& $\mathbf{0.983 \scriptstyle \pm 0.002}$ % EUBO d=200
\\
%%%%%%%%%%%%%%%%%%%%%%%%%%%%%%%%%%%%%%%%%%%%%%%%%%%%%%%%%%%%%%%%%%%%%%%%%%%%%%%%%%%%%%%%
& VarGrad
& $-3.73 \scriptstyle \pm 0.287$ % ELBO d=2
& $-43.533 \scriptstyle \pm 3.134$ % ELBO d=50
& $-210.878 \scriptstyle \pm 14.927$ % ELBO d=200
& $0.954 \scriptstyle \pm 0.008$ % EUBO d=2
& $0.985 \scriptstyle \pm 0.004$ % EUBO d=50
& $\mathbf{0.979 \scriptstyle \pm 0.008}$ % EUBO d=200
\\
\midrule
% %%%%%%%%%%%%%%%%%%%%%%%%%%%%%%%%%%%%%%%%%%%%%%%%%%%%%%%%%%%%%%%%%%%%%%%%%%%%%%%%%%%%%%%%
CMCD
& ELBO
& $\mathbf{-3.295 \scriptstyle \pm 0.162}$ % ELBO d=2
& $\mathbf{-13.176 \scriptstyle \pm 0.135}$ % ELBO d=50
& $\mathbf{-56.499 \scriptstyle \pm 3.139}$ % ELBO d=200
& $\mathbf{0.719 \scriptstyle \pm 0.025}$ % EUBO d=2
& $0.0 \scriptstyle \pm 0.0$ % EUBO d=50
& $0.0 \scriptstyle \pm 0.0$ % EUBO d=200
\\
%%%%%%%%%%%%%%%%%%%%%%%%%%%%%%%%%%%%%%%%%%%%%%%%%%%%%%%%%%%%%%%%%%%%%%%%%%%%%%%%%%%%%%%%
& VarGrad
& $-4.882 \scriptstyle \pm 0.304$ % ELBO d=2
& $-11199.27 \scriptstyle \pm 5658.388$ % ELBO d=50
& $-88696.432 \scriptstyle \pm 42.207$ % ELBO d=200
& $0.36 \scriptstyle \pm 0.07$ % EUBO d=2
& $\mathbf{0.249 \scriptstyle \pm 0.43}$ % EUBO d=50
& $\mathbf{0.989 \scriptstyle \pm 0.001}$ % EUBO d=200
\\
\bottomrule
% %%%%%%%%%%%%%%%%%%%%%%%%%%%%%%%%%%%%%%%%%%%%%%%%%%%%%%%%%%%%%%%%%%%%%%%%%%%%%%%%%%%%%%%%
\end{tabular}
}}
\end{sc}
\end{small}
\end{center}
\vskip -0.1in
\caption{ELBO and EMC values for different loss functions, that is, ELBO and VarGrad \cite{richter2020vargrad} on the MoG target.}
\label{abl_loss}
\end{table*}
%%%%%%%%%%%%%%%%%%%%%%%%%%%%%%%%%%%%%%%%%%%%%%%%%%%%%%%%%%%%%%%%%%%%%%%%%%%%%
