# Supplementary material for: Beyond ELBOs: A Large-Scale Evaluation of Variational Methods for Sampling
Source: arXiv:2406.07423 source file (2024-06-11)
Supplement: Supplementary file 3 [file hparam_table_old.tex]

\newpage

\begin{table}[hbtp]
\centering


\resizebox{\textwidth}{!}{  

\begin{tabular}{l|c|ccccccccc}
	\toprule 
         \textbf{Methods} / Parameters   & Grid 
         & Funnel & GMM  & STMM  & BMM  & ManyWell  & Reacher & Nice & - & ADLP \\
        %%%%%%%%%%%%%%%%%%%%%%%%%%%%%%%%%%%%%%%%%%%%%%%%%%%%%%%%%%%%%%%%%%%%%%%%%%%%%%%%%
        \midrule
        \textbf{MFVI}  & \\
        Initial Scale   & \{0.1, 1, 10\} & 1 & 10 & 10 & 0.1 & 0.1 & 0.1 & 10 & - & -\\
        Learning Rate   & $\{ 10^{-2},10^{-3},10^{-4},10^{-5} \}$ & $10^{-2}$ & $10^{-3}$ & $10^{-3}$ & $10^{-2}$ & $10^{-4}$ & $10^{-3}$  & $10^{-3}$ & - & -\\
        %%%%%%%%%%%%%%%%%%%%%%%%%%%%%%%%%%%%%%%%%%%%%%%%%%%%%%%%%%%%%%%%%%%%%%%%%%%%%%%%%
        \midrule
        \textbf{GMMVI}  & \\
        Initial Scale  & \{0.1, 1, 10\} & 0.1 & 10 & 10 & 10 & 10 & 0.1 & -  & - & -\\
        % Prior Scale & \{0.1, 1, 10\} & 0.1 & - & - & - & - & - & -  & - & -\\
        %%%%%%%%%%%%%%%%%%%%%%%%%%%%%%%%%%%%%%%%%%%%%%%%%%%%%%%%%%%%%%%%%%%%%%%%%%%%%%%%%
        \midrule
        \textbf{NFVI}  & \\
        Initial Scale   & \{0.1, 1, 10\} & - & - & - & - & - & - & - & - & -\\
        Learning Rate   & $\{10^{-3},10^{-4},10^{-5} \}$ & - & - & - & - & - & - & - & - & -\\
        % Flow Type & \{\} & - & - & - & - & - & - & - & - & -\\
        Num. Flows & \{\} & - & - & - & - & - & - & - & - & -\\
        %%%%%%%%%%%%%%%%%%%%%%%%%%%%%%%%%%%%%%%%%%%%%%%%%%%%%%%%%%%%%%%%%%%%%%%%%%%%%%%%%
        \midrule
        \textbf{SMC}  & \\
        Initial Scale   & \{0.1, 1, 10\} & 1 & 10 & 10 & 1 & 1 & 0.1 & 1 & - & -\\
        HMC stepsize ($\beta \leq 0.5$) & \{0.001, 0.01, 0.05, 0.1, 0.2\}  &  0.001 & 0.2 & 0.2 & 0.1 & 0.2 & 0.01 & 0.1 & - & - \\
        HMC stepsize ($\beta > 0.5$) & \{0.001, 0.01, 0.05, 0.1, 0.2\}  & 0.1 & 0.2 & 0.2 & 0.05 & 0.001 & 0.1 & 0.1 & - & -\\
        %%%%%%%%%%%%%%%%%%%%%%%%%%%%%%%%%%%%%%%%%%%%%%%%%%%%%%%%%%%%%%%%%%%%%%%%%%%%%%%%%
        \midrule
        \textbf{AFT}  & \\
        Initial Scale   & \{0.1, 1, 10\} & 1 & 10 & 10 & 1 & 1 & 0.1 & 1 & - & -\\
        Learning Rate   & $\{ 10^{-3},10^{-4},10^{-5} \}$ & $10^{-3}$ & $10^{-3}$ & $10^{-3}$ & $10^{-4}$ & $10^{-3}$ & $10^{-3}$ & $10^{-3}$ & - & -\\
        % Flow Type & \{\} & - & - & - & - & - & - & - & - & -\\
        %%%%%%%%%%%%%%%%%%%%%%%%%%%%%%%%%%%%%%%%%%%%%%%%%%%%%%%%%%%%%%%%%%%%%%%%%%%%%%%%%
        \midrule
        \textbf{CRAFT/SNF}  & \\
        Initial Scale   & \{0.1, 1, 10\} & 1 & 10 & 10 & 0.1 & 1 & - & 1 & - & -\\
        Learning Rate   & $\{ 10^{-3},10^{-4},10^{-5} \}$ & $10^{-3}$ & $10^{-4}$ & $10^{-4}$ & $10^{-4}$ & $10^{-4}$ & $10^{-3}$ & $10^{-3}$ & - & -\\
        % Flow Type & \{\} & - & - & - & - & - & - & - & - & -\\
        %%%%%%%%%%%%%%%%%%%%%%%%%%%%%%%%%%%%%%%%%%%%%%%%%%%%%%%%%%%%%%%%%%%%%%%%%%%%%%%%%
        \midrule
        \textbf{FAB}  & \\
        Initial Scale   & \{0.1, 1, 10\} & - & - & - & - & - & - & - & - & -\\
        %%%%%%%%%%%%%%%%%%%%%%%%%%%%%%%%%%%%%%%%%%%%%%%%%%%%%%%%%%%%%%%%%%%%%%%%%%%%%%%%%
        % \textbf{SNF}  & \\
        % Initial Scale   & \{0.1, 1, 10\} & 1 & - & - & - & - & - & - & - & -\\
        % Learning Rate   & $\{ 10^{-3},10^{-4},10^{-5} \}$ & $10^{-3}$ & - & - & - & - & - & - & - & -\\
        % Flow Type & \{\} & - & - & - & - & - & - & - & - & -\\
        %%%%%%%%%%%%%%%%%%%%%%%%%%%%%%%%%%%%%%%%%%%%%%%%%%%%%%%%%%%%%%%%%%%%%%%%%%%%%%%%%
        \midrule
        \textbf{DDS}  & \\
        Initial Scale   & \{0.1, 1, 10\} & - & - & - & - & - & - & - & - & -\\
        Learning Rate   & $\{ 10^{-3},10^{-4},10^{-5} \}$ & - & - & - & - & - & - & - & - & -\\        %%%%%%%%%%%%%%%%%%%%%%%%%%%%%%%%%%%%%%%%%%%%%%%%%%%%%%%%%%%%%%%%%%%%%%%%%%%%%%%%%
        \midrule
        \textbf{PIS}  & \\
        Learning Rate   & $\{ 10^{-3},10^{-4},10^{-5} \}$ & $10^{-3}$ & $10^{-3}$ & $10^{-3}$ & $10^{-4}$ & $10^{-3}$ & $10^{-5}$ & $10^{-3}$  & - & -\\        %%%%%%%%%%%%%%%%%%%%%%%%%%%%%%%%%%%%%%%%%%%%%%%%%%%%%%%%%%%%%%%%%%%%%%%%%%%%%%%%%
        % \midrule
        % \textbf{ULA}  & \\
        % Initial Scale   & \{0.1, 1, 10\} & 1 & 0.1 & - & - & - & - & - & - & -\\
        % Learning Rate & $\{ 10^{-3},10^{-4},10^{-5} \}$ & $10^{-3}$ & $10^{-3}$ & - & - & - & - & - & - & -\\
        % $q_0$ trainable & \{\text{True, False}\} & True & True & - & - & - & - & - & - & -\\
        % %%%%%%%%%%%%%%%%%%%%%%%%%%%%%%%%%%%%%%%%%%%%%%%%%%%%%%%%%%%%%%%%%%%%%%%%%%%%%%%%%
        \midrule
        \textbf{UHA/LDVI}  & \\
        Initial Scale   & \{0.1, 1, 10\} & 1 & 10 & 1 & 0.1 & 0.1 & - & 0.1 & - & -\\
        Learning Rate & $\{ 10^{-3},10^{-4},10^{-5} \}$ & $10^{-4}$ & $10^{-3}$ & $10^{-3}$ & $10^{-3}$ & $10^{-3}$ & - & $10^{-3}$ & - & -\\
        % $q_0$ trainable & \{\text{True, False}\} & True & True & True & True & - & - & True & - & -\\
        %%%%%%%%%%%%%%%%%%%%%%%%%%%%%%%%%%%%%%%%%%%%%%%%%%%%%%%%%%%%%%%%%%%%%%%%%%%%%%%%%
        \midrule
        \textbf{ULA/MCD}  & \\
        Initial Scale   & \{0.1, 1, 10\} & 1 & 0.1 & 1 & 1 & 0.1 & - & 10 & - & -\\
        Learning Rate & $\{ 10^{-3},10^{-4},10^{-5} \}$ & $10^{-3}$ & $10^{-3}$ & $10^{-3}$ & $10^{-3}$ & $10^{-3}$ & - &  $10^{-3}$ & - & -\\
        % $q_0$ trainable & \{\text{True, False}\} & True & True & True & True & - & - & True & - & -\\
        %%%%%%%%%%%%%%%%%%%%%%%%%%%%%%%%%%%%%%%%%%%%%%%%%%%%%%%%%%%%%%%%%%%%%%%%%%%%%%%%%
        \midrule
        \textbf{CMCD}  & \\
        Initial Scale   & \{0.1, 1, 10\} & 1 & 1 & 10 & - & 1 & - & 10 & - & -\\
        Learning Rate & $\{ 10^{-3},10^{-4},10^{-5} \}$ & $10^{-3}$ & $10^{-3}$ & $10^{-3}$ & - & $10^{-3}$ & - & $10^{-3}$ & - & -\\
        % $q_0$ trainable & \{\text{True, False}\} & - & - & - & - & - & - & - & - & -\\
        %%%%%%%%%%%%%%%%%%%%%%%%%%%%%%%%%%%%%%%%%%%%%%%%%%%%%%%%%%%%%%%%%%%%%%%%%%%%%%%%%
	\bottomrule
\end{tabular}
}
 \caption{Hyperparameter Selection for all VI algorithms. The `Grid' column indicates the values over which we performed a grid search. The values in the column which are marked with experiment names indicate which values were chosen for the reported results.}\label{hparams}
\vskip -0.15in
\end{table}

%%%%%%%%%%%%%%%%%%%%%%%%%%%%%%%%%%%%%%%%%%%%%%%%%%%%%%%%%%%%%%%%%%%%%%%%%%%%%%%%%%%%%%%%%%
%%%%%%%%%%%%%%%%%%%%%%%%%%%%%%%%%%%%%%%%%%%%%%%%%%%%%%%%%%%%%%%%%%%%%%%%%%%%%%%%%%%%%%%%%%
%%%%%%%%%%%%%%%%%%%%%%%%%%%%%%%%%%%%%%%%%%%%%%%%%%%%%%%%%%%%%%%%%%%%%%%%%%%%%%%%%%%%%%%%%%

\newpage

\begin{table}[hbtp]
\centering


\resizebox{\textwidth}{!}{  

\begin{tabular}{l|c|ccccccccc}
	\toprule 
         \textbf{Methods} / Parameters   & Grid 
         & Credit & Cancer  & Brownian  & Sonar  & Seeds  & Ionosphere & LGCP & GMM40 & - \\
        %%%%%%%%%%%%%%%%%%%%%%%%%%%%%%%%%%%%%%%%%%%%%%%%%%%%%%%%%%%%%%%%%%%%%%%%%%%%%%%%%
        \midrule
        \textbf{MFVI}  & \\
        Initial Scale   & \{0.1, 1, 10\} & 0.1 & 10 & 1 & 0.1 & 1 & 1 & 0.1 & - & -\\
        Learning Rate   & $\{ 10^{-2},10^{-3},10^{-4},10^{-5} \}$ & $10^{-3}$ & $10^{-2}$ & $10^{-3}$ & $10^{-3}$ & $10^{-4}$ & $10^{-4}$ & $10^{-3}$ & $10^{-2}$ & -\\
        %%%%%%%%%%%%%%%%%%%%%%%%%%%%%%%%%%%%%%%%%%%%%%%%%%%%%%%%%%%%%%%%%%%%%%%%%%%%%%%%%
        \midrule
        \textbf{GMMVI}  & \\
        Initial Scale  & \{0.1, 1, 10\} & 0.1 & 1 & 0.1 & 1 & 0.1 & 10 & NA & - & -\\
        % Prior Scale & \{0.1, 1, 10\} & 0.1 & - & - & - & - & - & -  & - & -\\
        %%%%%%%%%%%%%%%%%%%%%%%%%%%%%%%%%%%%%%%%%%%%%%%%%%%%%%%%%%%%%%%%%%%%%%%%%%%%%%%%%
        \midrule
        \textbf{NFVI}  & \\
        Initial Scale   & \{0.1, 1, 10\} & - & - & - & - & - & - & - & - & -\\
        Learning Rate   & $\{ 10^{-3},10^{-4},10^{-5} \}$ & - & - & - & - & - & - & - & - & -\\
        % Flow Type & \{\} & - & - & - & - & - & - & - & - & -\\
        Num. Flows & \{4,8,16,32\} & - & - & - & - & - & - & - & - & -\\
        %%%%%%%%%%%%%%%%%%%%%%%%%%%%%%%%%%%%%%%%%%%%%%%%%%%%%%%%%%%%%%%%%%%%%%%%%%%%%%%%%
        \midrule
        \textbf{SMC}  & \\
        Initial Scale   & \{0.1, 1, 10\}& 0.1 & 1 & 1 & 1 & 1 & 1 & 1 & - & -\\
        HMC stepsize ($\beta \leq 0.5$) & \{0.001, 0.01, 0.05, 0.1, 0.2\} & 0.1 & 0.05 & 0.001 & 0.05 & 0.2 & 0.2 & 0.01 & 0.2& -\\
        HMC stepsize ($\beta > 0.5$) & \{0.001, 0.01, 0.05, 0.1, 0.2\} & 0.1 & 0.01 & 0.05 & 0.001 & 0.05 & 0.2 & 0.2 & 0.001 & -\\
        %%%%%%%%%%%%%%%%%%%%%%%%%%%%%%%%%%%%%%%%%%%%%%%%%%%%%%%%%%%%%%%%%%%%%%%%%%%%%%%%%
        \midrule
        \textbf{AFT}  & \\
        Initial Scale   & \{0.1, 1, 10\} & 0.1 & 0.1 & NA & 1 & 1 & 1 & 1 & - & - \\
        Learning Rate   & $\{ 10^{-3},10^{-4},10^{-5} \}$ & $10^{-3}$ & $10^{-3}$ & NA & $10^{-3}$ & $10^{-4}$ & $10^{-3}$ & $10^{-3}$ & $10^{-3}$ & -\\
        % Flow Type & \{\} & - & - & - & - & - & - & - & - & -\\
        %%%%%%%%%%%%%%%%%%%%%%%%%%%%%%%%%%%%%%%%%%%%%%%%%%%%%%%%%%%%%%%%%%%%%%%%%%%%%%%%%
        \midrule
        \textbf{CRAFT/SNF}  & \\
        Initial Scale   & \{0.1, 1, 10\} & 0.1 & 1 & 
1 & 1 &  0.1 & 0.1 & 1 & - & -\\
        Learning Rate   & $\{ 10^{-3},10^{-4},10^{-5} \}$ & $10^{-4}$ & $10^{-3}$ & $10^{-3}$ & $10^{-3}$ & $10^{-3}$ & $10^{-3}$ & $10^{-3}$ & $10^{-3}$ & -\\
        % Flow Type & \{\} & - & - & - & - & - & - & - & - & -\\
        %%%%%%%%%%%%%%%%%%%%%%%%%%%%%%%%%%%%%%%%%%%%%%%%%%%%%%%%%%%%%%%%%%%%%%%%%%%%%%%%%
        \midrule
        \textbf{FAB}  & \\
        Initial Scale   & \{0.1, 1, 10\} & - & - & - & - & - & - & - & - & -\\
        Learning Rate   & $\{ 10^{-3},10^{-4},10^{-5} \}$ & - & - & - & - & - & - & - & - & -\\
        % Flow Type & \{\} & - & - & - & - & - & - & - & - & -\\
        %%%%%%%%%%%%%%%%%%%%%%%%%%%%%%%%%%%%%%%%%%%%%%%%%%%%%%%%%%%%%%%%%%%%%%%%%%%%%%%%%
        % \textbf{SNF}  & \\
        % Initial Scale   & \{0.1, 1, 10\} & 1 & - & - & - & - & - & - & - & -\\
        % Learning Rate   & $\{ 10^{-3},10^{-4},10^{-5} \}$ & $10^{-3}$ & - & - & - & - & - & - & - & -\\
        % Flow Type & \{\} & - & - & - & - & - & - & - & - & -\\
        %%%%%%%%%%%%%%%%%%%%%%%%%%%%%%%%%%%%%%%%%%%%%%%%%%%%%%%%%%%%%%%%%%%%%%%%%%%%%%%%%
        \midrule
        \textbf{DDS}  & \\
        Initial Scale   & \{0.1, 1, 10\} & - & - & - & - & - & - & - & - & -\\
        Learning Rate   & $\{ 10^{-3},10^{-4},10^{-5} \}$ & - & - & - & - & - & - & - & - & -\\        %%%%%%%%%%%%%%%%%%%%%%%%%%%%%%%%%%%%%%%%%%%%%%%%%%%%%%%%%%%%%%%%%%%%%%%%%%%%%%%%%
        \midrule
        \textbf{PIS}  & \\
        Learning Rate   & $\{ 10^{-3},10^{-4},10^{-5} \}$ & $10^{-4}$ & $10^{-4}$ & $10^{-4}$ & $10^{-3}$ & $10^{-3}$ & $10^{-4}$ & Prob & $10^{-3}$ & -\\ 
       %%%%%%%%%%%%%%%%%%%%%%%%%%%%%%%%%%%%%%%%%%%%%%%%%%%%%%%%%%%%%%%%%%%%%%%%%%%%%%%%%
        % \midrule
        % \textbf{ULA}  & \\
        % Initial Scale   & \{0.1, 1, 10\} & 1 & 0.1 & - & - & - & - & - & - & -\\
        % Learning Rate & $\{ 10^{-3},10^{-4},10^{-5} \}$ & $10^{-3}$ & $10^{-3}$ & - & - & - & - & - & - & -\\
        % $q_0$ trainable & \{\text{True, False}\} & True & True & - & - & - & - & - & - & -\\
        % %%%%%%%%%%%%%%%%%%%%%%%%%%%%%%%%%%%%%%%%%%%%%%%%%%%%%%%%%%%%%%%%%%%%%%%%%%%%%%%%%
        \midrule
        \textbf{UHA/LDVI}  & \\
        Initial Scale   & \{0.1, 1, 10\} & 0.1 & 0.1 & 1 & 1 & 0.1 & 0.1 & 0.1 & - & -\\
        Learning Rate   & $\{ 10^{-3},10^{-4},10^{-5} \}$ & $10^{-3}$ & $10^{-3}$ & $10^{-3}$ & $10^{-3}$ & $10^{-3}$ & $10^{-3}$ & $10^{-3}$ & $10^{-3}$ & -\\
        % $q_0$ trainable & \{\text{True, False}\} & - & - & - & - & - & - & - & - & -\\
        %%%%%%%%%%%%%%%%%%%%%%%%%%%%%%%%%%%%%%%%%%%%%%%%%%%%%%%%%%%%%%%%%%%%%%%%%%%%%%%%%
        \midrule
        \textbf{ULA/MCD}  & \\
        Initial Scale   & \{0.1, 1, 10\} & 0.1 & 0.1 & 1 & 0.1 & 0.1 & 1 & 1 & - & -\\
        Learning Rate   & $\{ 10^{-3},10^{-4},10^{-5} \}$ & $10^{-4}$ & $10^{-3}$ & $10^{-3}$ & $10^{-3}$ & $10^{-3}$ & $10^{-3}$ & $10^{-3}$ & $10^{-3}$ & -\\
        % $q_0$ trainable & \{\text{True, False}\} & - & - & - & - & - & - & - & - & -\\
        %%%%%%%%%%%%%%%%%%%%%%%%%%%%%%%%%%%%%%%%%%%%%%%%%%%%%%%%%%%%%%%%%%%%%%%%%%%%%%%%%
        \midrule
        \textbf{CMCD}  & \\
        Initial Scale   & \{0.1, 1, 10\} & P & 0.1 & 0.1 & 0.1 & 0.1 & 1 & 1 & - & -\\
        Learning Rate & $\{ 10^{-3},10^{-4},10^{-5} \}$ & - & $10^{-3}$ & $10^{-3}$ & $10^{-3}$ & $10^{-3}$ & $10^{-3}$ & $10^{-3}$ & $10^{-3}$ & -\\
        % $q_0$ trainable & \{\text{True, False}\} & - & - & - & - & - & - & - & - & -\\
        %%%%%%%%%%%%%%%%%%%%%%%%%%%%%%%%%%%%%%%%%%%%%%%%%%%%%%%%%%%%%%%%%%%%%%%%%%%%%%%%%
	\bottomrule
\end{tabular}
}
 \caption{Hyperparameter Selection for all VI algorithms. The `Grid' column indicates the values over which we performed a grid search. The values in the column which are marked with experiment names indicate which values were chosen for the reported results.}\label{hparams2}
\vskip -0.15in
\end{table}

%%%%%%%%%%%%%%%%%%%%%%%%%%%%%%%%%%%%%%%%%%%%%%%%%%%%%%%%%%%%%%%%%%%%%%%%%%%%%%%%%%%%%%%%%%
%%%%%%%%%%%%%%%%%%%%%%%%%%%%%%%%%%%%%%%%%%%%%%%%%%%%%%%%%%%%%%%%%%%%%%%%%%%%%%%%%%%%%%%%%%
%%%%%%%%%%%%%%%%%%%%%%%%%%%%%%%%%%%%%%%%%%%%%%%%%%%%%%%%%%%%%%%%%%%%%%%%%%%%%%%%%%%%%%%%%%

\newpage

\begin{table}[hbtp]
\centering


\resizebox{\textwidth}{!}{  

\begin{tabular}{l|c|ccccccccc}
	\toprule 
         \textbf{Methods} / Parameters   & Grid 
         & GMM40 & GMM  & STMM  & BMM  & NICE  & - & - & - & - \\
        %%%%%%%%%%%%%%%%%%%%%%%%%%%%%%%%%%%%%%%%%%%%%%%%%%%%%%%%%%%%%%%%%%%%%%%%%%%%%%%%%
        \midrule
        \textbf{MFVI}  & \\
        Learning Rate   & $\{ 10^{-2},10^{-3},10^{-4},10^{-5} \}$ & $10^{-2}$ & $10^{-3}$ & $10^{-3}$  & $10^{-3}$  & $10^{-3}$ & - & - & - & -\\

        %%%%%%%%%%%%%%%%%%%%%%%%%%%%%%%%%%%%%%%%%%%%%%%%%%%%%%%%%%%%%%%%%%%%%%%%%%%%%%%%%
        \midrule
        \textbf{NFVI}  & \\
        Learning Rate   & $\{ 10^{-3},10^{-4},10^{-5} \}$ & - & - & - & - & - & - & - & - & -\\
        % Flow Type & \{\} & - & - & - & - & - & - & - & - & -\\
        Num. Flows & \{4,8,16,32\} & - & - & - & - & - & - & - & - & -\\
        %%%%%%%%%%%%%%%%%%%%%%%%%%%%%%%%%%%%%%%%%%%%%%%%%%%%%%%%%%%%%%%%%%%%%%%%%%%%%%%%%
        \midrule
        \textbf{SMC}  & \\
        HMC stepsize ($\beta \leq 0.5$) & \{0.001, 0.01, 0.05, 0.1, 0.2\} & 0.2 & 0.2 & 0.2 & 0.2 & 0.2 & - & - & - & -\\
        HMC stepsize ($\beta > 0.5$) & \{0.001, 0.01, 0.05, 0.1, 0.2\}& 0.001 & 0.2 & 0.2 & 0.001 &  0.1  & - & - & - & -\\
        %%%%%%%%%%%%%%%%%%%%%%%%%%%%%%%%%%%%%%%%%%%%%%%%%%%%%%%%%%%%%%%%%%%%%%%%%%%%%%%%%
        \midrule
        \textbf{AFT}  & \\
        Learning Rate   & $\{ 10^{-3},10^{-4},10^{-5} \}$ & $10^{-3}$ & $10^{-3}$ & $10^{-4}$ & $10^{-4}$  & $10^{-3}$ & - & - & - & -\\
        % Flow Type & \{\} & - & - & - & - & - & - & - & - & -\\
        %%%%%%%%%%%%%%%%%%%%%%%%%%%%%%%%%%%%%%%%%%%%%%%%%%%%%%%%%%%%%%%%%%%%%%%%%%%%%%%%%
        \midrule
        \textbf{CRAFT/SNF}  & \\
        Learning Rate   & $\{ 10^{-3},10^{-4},10^{-5} \}$ & $10^{-3}$ & $10^{-3}$ & $10^{-4}$ & $10^{-3}$  & $10^{-3}$ & - & - & - & -\\
        % Flow Type & \{\} & - & - & - & - & - & - & - & - & -\\
        %%%%%%%%%%%%%%%%%%%%%%%%%%%%%%%%%%%%%%%%%%%%%%%%%%%%%%%%%%%%%%%%%%%%%%%%%%%%%%%%%
        \midrule
        \textbf{FAB}  & \\
        Learning Rate   & $\{ 10^{-3},10^{-4},10^{-5} \}$ & - & - & - & - & - & - & - & - & -\\
        % Flow Type & \{\} & - & - & - & - & - & - & - & - & -\\
        %%%%%%%%%%%%%%%%%%%%%%%%%%%%%%%%%%%%%%%%%%%%%%%%%%%%%%%%%%%%%%%%%%%%%%%%%%%%%%%%%
        % \textbf{SNF}  & \\
        % Initial Scale   & \{0.1, 1, 10\} & 1 & - & - & - & - & - & - & - & -\\
        % Learning Rate   & $\{ 10^{-3},10^{-4},10^{-5} \}$ & $10^{-3}$ & - & - & - & - & - & - & - & -\\
        % Flow Type & \{\} & - & - & - & - & - & - & - & - & -\\
        %%%%%%%%%%%%%%%%%%%%%%%%%%%%%%%%%%%%%%%%%%%%%%%%%%%%%%%%%%%%%%%%%%%%%%%%%%%%%%%%%
        \midrule
        \textbf{DDS}  & \\
        Learning Rate   & $\{ 10^{-3},10^{-4},10^{-5} \}$ & - & - & - & - & - & - & - & - & -\\
        \midrule
        \textbf{PIS}  & \\
        Learning Rate   & $\{ 10^{-3},10^{-4},10^{-5} \}$ & $10^{-3}$ & $10^{-3}$ & $10^{-3}$ & $10^{-4}$ & $10^{-3}$ & - & - & - & -\\
       %%%%%%%%%%%%%%%%%%%%%%%%%%%%%%%%%%%%%%%%%%%%%%%%%%%%%%%%%%%%%%%%%%%%%%%%%%%%%%%%%
        % \midrule
        % \textbf{ULA}  & \\
        % Initial Scale   & \{0.1, 1, 10\} & 1 & 0.1 & - & - & - & - & - & - & -\\
        % Learning Rate   & $\{ 10^{-3},10^{-4},10^{-5} \}$ & - & - & - & - & - & - & - & - & -\\
        % $q_0$ trainable & \{\text{True, False}\} & True & True & - & - & - & - & - & - & -\\
        % %%%%%%%%%%%%%%%%%%%%%%%%%%%%%%%%%%%%%%%%%%%%%%%%%%%%%%%%%%%%%%%%%%%%%%%%%%%%%%%%%
        \midrule
        \textbf{UHA/LDVI}  & \\
        Learning Rate   & $\{ 10^{-3},10^{-4},10^{-5} \}$ & $10^{-3}$ & $10^{-3}$ & $10^{-3}$ & P & $10^{-3}$ & - & - & - & -\\
        % $q_0$ trainable & \{\text{True, False}\} & - & - & - & - & - & - & - & - & -\\
        %%%%%%%%%%%%%%%%%%%%%%%%%%%%%%%%%%%%%%%%%%%%%%%%%%%%%%%%%%%%%%%%%%%%%%%%%%%%%%%%%
        \midrule
        \textbf{ULA/MCD}  & \\
        Learning Rate   & $\{ 10^{-3},10^{-4},10^{-5} \}$ & $10^{-3}$ & $10^{-3}$ & $10^{-3}$ & P & $10^{-3}$ & - & - & - & -\\
        % $q_0$ trainable & \{\text{True, False}\} & - & - & - & - & - & - & - & - & -\\
        %%%%%%%%%%%%%%%%%%%%%%%%%%%%%%%%%%%%%%%%%%%%%%%%%%%%%%%%%%%%%%%%%%%%%%%%%%%%%%%%%
        \midrule
        \textbf{CMCD}  & \\
        Learning Rate   & $\{ 10^{-3},10^{-4},10^{-5} \}$ & $10^{-3}$ & $10^{-3}$ & $10^{-3}$ & P & $10^{-3}$  & - & - & - & -\\
        % $q_0$ trainable & \{\text{True, False}\} & - & - & - & - & - & - & - & - & -\\
        %%%%%%%%%%%%%%%%%%%%%%%%%%%%%%%%%%%%%%%%%%%%%%%%%%%%%%%%%%%%%%%%%%%%%%%%%%%%%%%%%
	\bottomrule
\end{tabular}
}
 \caption{Hyperparameter Selection for all VI algorithms. The `Grid' column indicates the values over which we performed a grid search. The values in the column which are marked with experiment names indicate which values were chosen for the reported results.}\label{hparams2}
\vskip -0.15in
\end{table}
